# Supplementary material for: HungerGist: An Interpretable Predictive Model for Food Insecurity
Source: arXiv:2311.10953 source file (2023-11-18)
Supplement: Supplementary file 1 [file 99_appendix.tex]

\appendix
\section{Appendix}
\subsection{Traditional factors}

% \begin{table*}[h]
% \centering
% \caption{\label{tab:data}
% \textbf{Data List.}
% }
